# Supplementary material for: First observation of correlations between spin and transverse momenta in back-to-back dihadron production at CLAS12
Source: arXiv:2208.05086 ancillary file (2022-08-10)
Supplement: Supplementary file 1 [file appendix.pdf]

# Ancillary files: First observation of correlations between spin and transverse momenta in back-to-back dihadron production at CLAS12


H. Avakian

*Thomas Jefferson National Accelerator Facility, Newport News, Virginia 23606*

T.B. Hayward[a]

*University of Connecticut, Storrs, Connecticut 06269*

A. Kotzinian

*Yerevan Physics Institute, 375036 Yerevan, Armenia and*

*INFN, Sezione di Torino, 10125 Torino, Italy*

(The CLAS Collaboration)



(Dated: August 9, 2022)



[a] timothy.hayward@uconn.edu

The beam-spin asymmetry that we measure is given in Ref. [1],

$$\mathcal{A}_{LU} = -\sqrt{1-\epsilon^2}\frac{\mathcal{F}_{LU}^{\sin\Delta\phi}}{\mathcal{F}_{UU}}\sin\Delta\phi, \tag{1}$$

where the $\epsilon$-dependent term in front of the ratio of structure functions describes the "depolarization" of the virtual photon compared to the original electron,

$$\epsilon = \frac{1-y-\frac{1}{4}\gamma^2y^2}{1-y+\frac{1}{2}y^2+\frac{1}{4}\gamma^2y^2}, \tag{2}$$

with $\gamma = 2m_N x/Q$. Additionally, the structure functions in the asymmetry definition can be expanded as,

$$-\sqrt{1-\epsilon^2}\frac{\mathcal{F}_{LU}^{\sin\Delta\phi}}{\mathcal{F}_{UU}}\sin\Delta\phi = -\sqrt{1-\epsilon^2}\frac{|\vec{P}_{T1}||\vec{P}_{T2}|}{m_N\,m_2}\frac{\mathcal{C}[w_5\,\hat{l}_1^{\perp h}D_1]}{\mathcal{C}[\hat{u}_1D_1]}\sin\Delta\phi\,. \tag{3}$$

Direct interpretation of the results in the context of the fracture and fragmentation functions will need to take into the account the transverse momentum dependent term in front of the convolutions. It is possible to include the depolarization factor and transverse momentum dependent terms on an event-by-event basis in our fit formalism. However, it has been explicitly checked that the difference between performing this event-by-event adjustment and taking the bin-by-bin average is negligible. As a result, in the tables below we report the measured beam-spin asymmetry given in Eq. 1 in order to to leave the asymmetries in the most basic possible form.

We impose the following kinematic constraints on our asymmetries (all definitions can be found in the main body of the Letter): $y < 0.75$, $0.2 < z_1 < 0.7$, $x_{F1} > 0$, $x_{F2} < 0$, $\Delta Y > 0$, $M_x > 0.90$ GeV and $M_{\pi p} > 1.5$ GeV. When asymmetries are reported with respect to $z_1$ we do not impose the $z_1$ requirement. When asymmetries are reported with respect to $x_{F2}$ or $\Delta Y$ we do not enforce the $x_{F1}$, $x_{F2}$ or $\Delta Y$ requirements. When asymmetries are reported with respect to $M_x$ we do not enforce the $M_x$ requirement.

A last remaining point concerns the overall sign of our asymmetries. Note the $-1$ that appears in front of Eq. 1. This, coupled with the ambiguity between whether $\Delta\phi$ is defined to be $\phi_1 - \phi_2$ or $\phi_2 - \phi_1$, causes the overall sign of our asymmetries to be meaningless. We have adopted the convention of including the $-1$ in Eq. 1 and have defined $\Delta\phi \equiv \phi_2 - \phi_1$, (the opposite of Ref. [1]). This causes the majority of our asymmetries to be negative.

### A. $x$-dependence of $\mathcal{A}_{LU}$

| Bin | $x$ Range | $< Q^2 >$ (GeV$^2$) | $< x >$ | $< y >$ | $< z_1 >$ | $< \zeta_2 >$ | $< P_{T1}P_{T2} >$ (GeV$^2$) | $< x_{F1} >$ | $< x_{F2} >$ | $< \Delta Y >$ |
|---|---|---|---|---|---|---|---|---|---|---|
| 1 | [0.0, 0.1] | 1.332 | 0.095 | 0.722 | 0.318 | 0.572 | 0.219 | 0.222 | -0.306 | 1.322 |
| 2 | (0.1, 0.2] | 1.969 | 0.156 | 0.652 | 0.337 | 0.571 | 0.194 | 0.237 | -0.319 | 1.351 |
| 3 | (0.2, 0.3] | 2.884 | 0.243 | 0.610 | 0.348 | 0.547 | 0.168 | 0.244 | -0.323 | 1.351 |
| 4 | (0.3, 0.4] | 4.098 | 0.339 | 0.619 | 0.347 | 0.501 | 0.155 | 0.241 | -0.317 | 1.312 |
| 5 | (0.4, 0.5] | 5.479 | 0.435 | 0.646 | 0.345 | 0.448 | 0.146 | 0.236 | -0.302 | 1.248 |
| 6 | (0.5, 0.6] | 6.880 | 0.524 | 0.671 | 0.345 | 0.394 | 0.134 | 0.233 | -0.271 | 1.164 |

TABLE I: Average kinematic values for the 1-D bins of $x$.

| Bin | $< x >$ | $\mathcal{A}_{LU}^{\sin(\Delta\phi)}$ | $\mathcal{A}_{LU}^{\sin(2\Delta\phi)}$ |
|---|---|---|---|
| 1 | 0.095 | $-0.007^{\pm0.009}_{\pm0.007}$ | $0.016^{\pm0.009}_{\pm0.007}$ |
| 2 | 0.156 | $-0.015^{\pm0.001}_{\pm0.001}$ | $0.000^{\pm0.001}_{\pm0.001}$ |
| 3 | 0.243 | $-0.020^{\pm0.002}_{\pm0.001}$ | $0.001^{\pm0.001}_{\pm0.001}$ |
| 4 | 0.339 | $-0.021^{\pm0.003}_{\pm0.002}$ | $0.003^{\pm0.003}_{\pm0.002}$ |
| 5 | 0.435 | $-0.032^{\pm0.007}_{\pm0.005}$ | $-0.013^{\pm0.006}_{\pm0.005}$ |
| 6 | 0.524 | $-0.017^{\pm0.031}_{\pm0.021}$ | $0.008^{\pm0.024}_{\pm0.017}$ |

TABLE II: The mean value of $x$ and the final beam-spin asymmetries as a function of $x$ in each bin. Asymmetries are given as ${\mathcal{A}_{LU}}^{\Delta_{\text{stat}}}_{\Delta_{\text{sys}}}$.

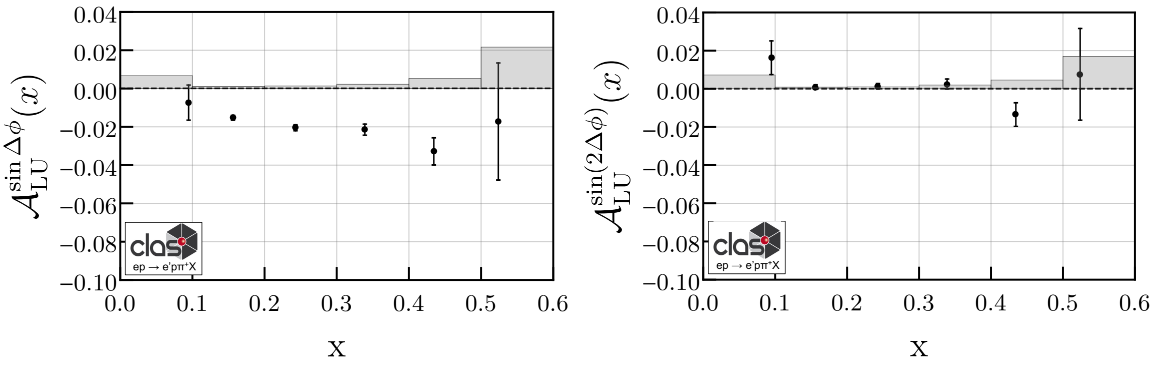


FIG. 1: The extracted amplitudes of the $\sin(\Delta\phi)$ and $\sin(2\Delta\phi)$ beam-spin asymmetries as a function of $x$.

### B. $z_1$-dependence of $\mathcal{A}_{LU}$

| Bin | $x$ Range | $< Q^2 >$ (GeV$^2$) | $< x >$ | $< y >$ | $< z_1 >$ | $< \zeta_2 >$ | $< P_{T1}P_{T2} >$ (GeV$^2$) | $< x_{F1} >$ | $< x_{F2} >$ | $< \Delta Y >$ |
|---|---|---|---|---|---|---|---|---|---|---|
| 1 | [0.1, 0.2] | 2.543 | 0.187 | 0.698 | 0.185 | 0.579 | 0.194 | 0.080 | -0.371 | 0.950 |
| 2 | (0.2, 0.3] | 2.628 | 0.209 | 0.649 | 0.254 | 0.562 | 0.187 | 0.145 | -0.340 | 1.113 |
| 3 | (0.3, 0.4] | 2.696 | 0.224 | 0.624 | 0.346 | 0.546 | 0.179 | 0.244 | -0.312 | 1.355 |
| 4 | (0.4, 0.5] | 2.681 | 0.223 | 0.622 | 0.444 | 0.538 | 0.171 | 0.349 | -0.299 | 1.603 |
| 5 | (0.5, 0.6] | 2.533 | 0.211 | 0.619 | 0.534 | 0.538 | 0.157 | 0.445 | -0.299 | 1.836 |
| 6 | (0.6, 0.7] | 2.181 | 0.194 | 0.580 | 0.619 | 0.542 | 0.102 | 0.538 | -0.307 | 2.149 |

TABLE III: Average kinematic values for the bins of $z_1$.

| Bin | $< z_1 >$ | $\mathcal{A}_{LU}^{\sin(\Delta\phi)}$ | $\mathcal{A}_{LU}^{\sin(2\Delta\phi)}$ |
|---|---|---|---|
| 1 | 0.185 | $-0.018^{\pm 0.005}_{\pm 0.001}$ | $-0.004^{\pm 0.005}_{\pm 0.001}$ |
| 2 | 0.253 | $-0.016^{\pm 0.002}_{\pm 0.001}$ | $0.000^{\pm 0.001}_{\pm 0.001}$ |
| 3 | 0.346 | $-0.022^{\pm 0.005}_{\pm 0.001}$ | $0.002^{\pm 0.001}_{\pm 0.001}$ |
| 4 | 0.444 | $-0.018^{\pm 0.002}_{\pm 0.002}$ | $0.001^{\pm 0.002}_{\pm 0.001}$ |
| 5 | 0.534 | $-0.005^{\pm 0.004}_{\pm 0.003}$ | $0.006^{\pm 0.003}_{\pm 0.003}$ |
| 6 | 0.619 | $0.001^{\pm 0.016}_{\pm 0.011}$ | $-0.008^{\pm 0.014}_{\pm 0.010}$ |

TABLE IV: The mean value of $z_1$ and the final beam-spin asymmetries as a function of $z_1$ in each bin. Asymmetries are given as $\mathcal{A}_{LU}{}^{\Delta_{\text{stat}}}_{\Delta_{\text{sys}}}$.

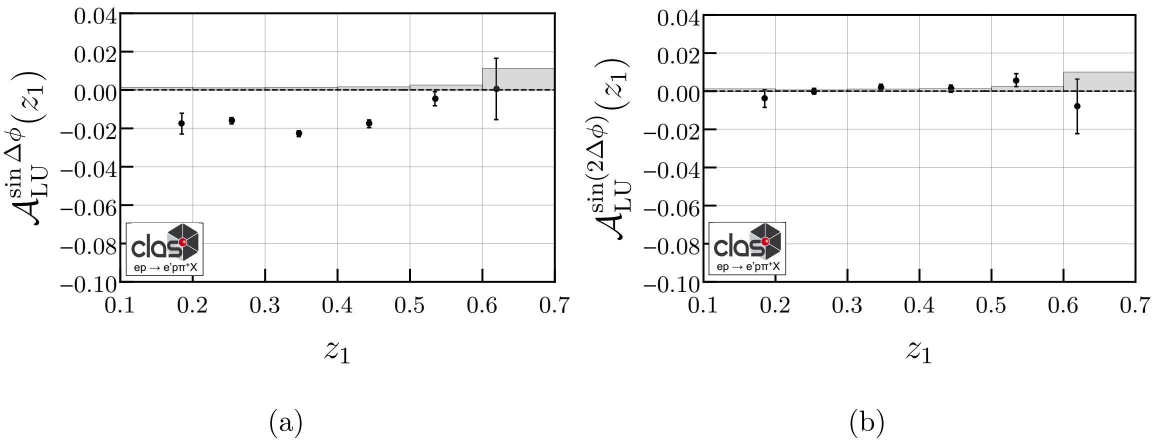


FIG. 2: The extracted amplitudes of the $\sin(\Delta\phi)$ and $\sin(2\Delta\phi)$ beam-spin asymmetries as a function of $z_1$.

### C. $\zeta_2$-dependence of $\mathcal{A}_{LU}$

| Bin | $x$ Range | $< Q^2 >$ (GeV$^2$) | $< x >$ | $< y >$ | $< z_1 >$ | $< \zeta_2 >$ | $< P_{T1}P_{T2} >$ (GeV$^2$) | $< x_{F1} >$ | $< x_{F2} >$ | $< \Delta Y >$ |
|---|---|---|---|---|---|---|---|---|---|---|
| 1 | [0.300, 0.383] | 6.516 | 0.479 | 0.696 | 0.383 | 0.370 | 0.111 | 0.253 | -0.153 | 0.996 |
| 2 | (0.383, 0.466] | 4.015 | 0.310 | 0.668 | 0.368 | 0.443 | 0.138 | 0.250 | -0.180 | 1.102 |
| 3 | (0.466, 0.549] | 2.806 | 0.230 | 0.635 | 0.351 | 0.513 | 0.170 | 0.243 | -0.255 | 1.243 |
| 4 | (0.549, 0.633] | 2.337 | 0.195 | 0.623 | 0.334 | 0.586 | 0.192 | 0.236 | -0.373 | 1.430 |
| 5 | (0.633, 0.716] | 2.079 | 0.171 | 0.629 | 0.318 | 0.660 | 0.202 | 0.232 | -0.493 | 1.625 |
| 6 | (0.716, 0.800] | 1.799 | 0.146 | 0.638 | 0.294 | 0.729 | 0.302 | 0.209 | -0.486 | 1.531 |

TABLE V: Average kinematic values for the bins of $\zeta_2$.

| Bin | $< \zeta_2 >$ | $\mathcal{A}_{LU}^{\sin(\Delta\phi)}$ | $\mathcal{A}_{LU}^{\sin(2\Delta\phi)}$ |
|---|---|---|---|
| 1 | 0.370 | $-0.031^{\pm 0.025}_{\pm 0.005}$ | $-0.001^{\pm 0.022}_{\pm 0.005}$ |
| 2 | 0.443 | $-0.021^{\pm 0.003}_{\pm 0.001}$ | $-0.005^{\pm 0.003}_{\pm 0.001}$ |
| 3 | 0.513 | $-0.019^{\pm 0.001}_{\pm 0.001}$ | $0.002^{\pm 0.001}_{\pm 0.001}$ |
| 4 | 0.586 | $-0.018^{\pm 0.002}_{\pm 0.001}$ | $0.000^{\pm 0.001}_{\pm 0.001}$ |
| 5 | 0.660 | $-0.007^{\pm 0.003}_{\pm 0.002}$ | $0.008^{\pm 0.003}_{\pm 0.002}$ |
| 6 | 0.729 | $0.016^{\pm 0.025}_{\pm 0.019}$ | $0.004^{\pm 0.020}_{\pm 0.016}$ |

TABLE VI: The mean value of $\zeta_2$ and the final beam-spin asymmetries as a function of $\zeta_2$ in each bin. Asymmetries are given as ${\mathcal{A}_{LU}}^{\Delta_{\rm stat}}_{\Delta_{\rm sys}}$.

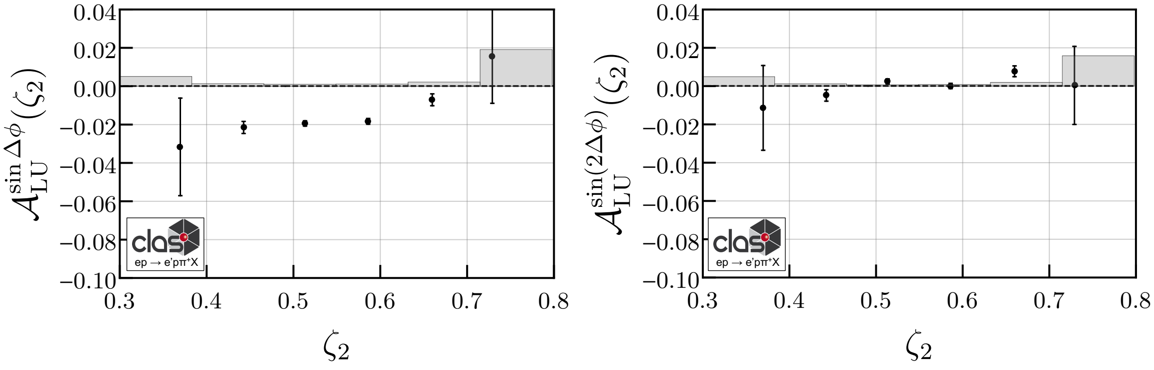


(a)

(b)

FIG. 3: The extracted amplitudes of the $\sin(\Delta\phi)$ and $\sin(2\Delta\phi)$ beam-spin asymmetries as a function of $\zeta_2$.

### D. $P_{T1}P_{T2}$-dependence of $\mathcal{A}_{LU}$

| Bin | $x$ Range | $< Q^2 >$ (GeV$^2$) | $< x >$ | $< y >$ | $< z_1 >$ | $< \zeta_2 >$ | $< P_{T1}P_{T2} >$ (GeV$^2$) | $< x_{F1} >$ | $< x_{F2} >$ | $< \Delta Y >$ |
|---|---|---|---|---|---|---|---|---|---|---|
| 1 | [0.0, 0.1] | 2.779 | 0.234 | 0.614 | 0.367 | 0.545 | 0.041 | 0.307 | -0.395 | 2.000 |
| 2 | (0.1, 0.2] | 2.672 | 0.220 | 0.628 | 0.347 | 0.548 | 0.100 | 0.266 | -0.364 | 1.572 |
| 3 | (0.2, 0.3] | 2.651 | 0.217 | 0.632 | 0.334 | 0.544 | 0.165 | 0.231 | -0.315 | 1.248 |
| 4 | (0.3, 0.4] | 2.644 | 0.215 | 0.635 | 0.327 | 0.546 | 0.231 | 0.206 | -0.273 | 1.034 |
| 5 | (0.4, 0.5] | 2.610 | 0.210 | 0.643 | 0.328 | 0.554 | 0.297 | 0.192 | -0.251 | 0.906 |
| 6 | (0.5, 0.6] | 2.555 | 0.202 | 0.651 | 0.333 | 0.565 | 0.363 | 0.183 | -0.236 | 0.820 |

TABLE VII: Average kinematic values for the bins of $P_{T1}P_{T2}$.

| Bin | $< P_{T1}P_{T2} >$ (GeV$^2$) | $\mathcal{A}_{LU}^{\sin(\Delta\phi)}$ | $\mathcal{A}_{LU}^{\sin(2\Delta\phi)}$ |
|---|---|---|---|
| 1 | 0.059 | $-0.010^{\pm 0.001}_{\pm 0.001}$ | $0.000^{\pm 0.001}_{\pm 0.001}$ |
| 2 | 0.147 | $-0.017^{\pm 0.002}_{\pm 0.002}$ | $-0.001^{\pm 0.001}_{\pm 0.001}$ |
| 3 | 0.244 | $-0.030^{\pm 0.003}_{\pm 0.003}$ | $-0.005^{\pm 0.002}_{\pm 0.001}$ |
| 4 | 0.343 | $-0.047^{\pm 0.005}_{\pm 0.004}$ | $-0.011^{\pm 0.004}_{\pm 0.003}$ |
| 5 | 0.442 | $-0.035^{\pm 0.010}_{\pm 0.007}$ | $0.006^{\pm 0.007}_{\pm 0.005}$ |
| 6 | 0.542 | $-0.040^{\pm 0.022}_{\pm 0.017}$ | $-0.001^{\pm 0.016}_{\pm 0.012}$ |

TABLE VIII: The mean value of $P_{T1}P_{T2}$ and the final beam-spin asymmetries as a function of $P_{T1}P_{T2}$ in each bin. Asymmetries are given as $\mathcal{A}_{LU}{}^{\Delta_{\rm stat}}_{\Delta_{\rm sys}}$.

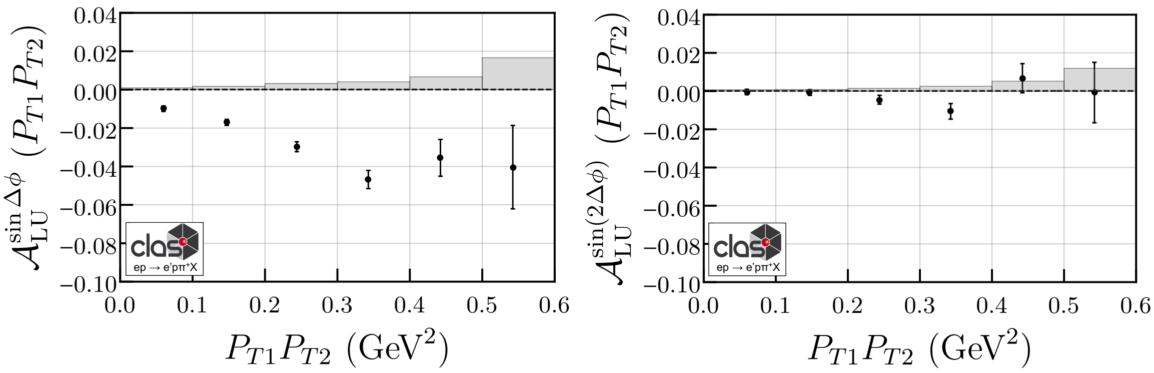


(a) (b)

FIG. 4: The extracted amplitudes of the $\sin(\Delta\phi)$ and $\sin(2\Delta\phi)$ beam-spin asymmetries as a function of $P_{T1}P_{T2}$.

### E. Multidimensional $P_{T1}P_{T2}$-dependence of $\mathcal{A}_{LU}$ with $0.2 \leq z_1 \leq 0.3$

| Bin | $x$ Range | $< Q^2 >$ (GeV$^2$) | $< x >$ | $< y >$ | $< z_1 >$ | $< \zeta_2 >$ | $< P_{T1}P_{T2} >$ (GeV$^2$) | $< x_{F1} >$ | $< x_{F2} >$ | $< \Delta Y >$ |
|---|---|---|---|---|---|---|---|---|---|---|
| 1 | [0.1, 0.2] | 2.677 | 0.213 | 0.648 | 0.257 | 0.576 | 0.043 | 0.201 | -0.474 | 1.834 |
| 2 | (0.2, 0.3] | 2.589 | 0.206 | 0.650 | 0.254 | 0.567 | 0.101 | 0.171 | -0.419 | 1.403 |
| 3 | (0.3, 0.4] | 2.638 | 0.212 | 0.644 | 0.253 | 0.551 | 0.166 | 0.145 | -0.336 | 1.065 |
| 4 | (0.4, 0.5] | 2.681 | 0.216 | 0.642 | 0.251 | 0.549 | 0.231 | 0.126 | -0.273 | 0.844 |
| 5 | (0.5, 0.6] | 2.652 | 0.211 | 0.648 | 0.252 | 0.559 | 0.297 | 0.111 | -0.244 | 0.714 |
| 6 | (0.6, 0.7] | 2.590 | 0.203 | 0.657 | 0.253 | 0.572 | 0.363 | 0.098 | -0.226 | 0.622 |

TABLE IX: Average kinematic values for the bins of $P_{T1}P_{T2}$ with $0.2 \leq z_1 \leq 0.3$.

| Bin | $< P_{T1}P_{T2} >$ (GeV$^2$) | $\mathcal{A}_{LU}^{\sin(\Delta\phi)}$ | $\mathcal{A}_{LU}^{\sin(2\Delta\phi)}$ |
|---|---|---|---|
| 1 | 0.063 | $-0.011^{\pm 0.003}_{\pm 0.001}$ | $-0.001^{\pm 0.003}_{\pm 0.001}$ |
| 2 | 0.149 | $-0.014^{\pm 0.003}_{\pm 0.002}$ | $-0.003^{\pm 0.003}_{\pm 0.001}$ |
| 3 | 0.244 | $-0.024^{\pm 0.004}_{\pm 0.003}$ | $-0.004^{\pm 0.004}_{\pm 0.002}$ |
| 4 | 0.342 | $-0.033^{\pm 0.007}_{\pm 0.004}$ | $-0.001^{\pm 0.006}_{\pm 0.003}$ |
| 5 | 0.441 | $-0.019^{\pm 0.014}_{\pm 0.009}$ | $0.017^{\pm 0.011}_{\pm 0.008}$ |
| 6 | 0.540 | $-0.057^{\pm 0.035}_{\pm 0.023}$ | $-0.040^{\pm 0.027}_{\pm 0.018}$ |

TABLE X: The mean value of $P_{T1}P_{T2}$ and the final beam-spin asymmetries as a function of $P_{T1}P_{T2}$ with $0.2 \leq z_1 \leq 0.3$ in each bin. Asymmetries are given as $\mathcal{A}_{LU}{}^{\Delta_{\text{stat}}}_{\Delta_{\text{sys}}}$.

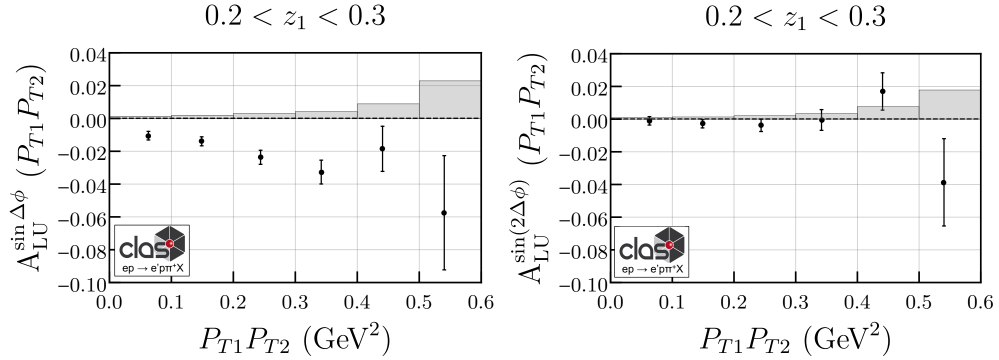


FIG. 5: The extracted amplitudes of the $\sin(\Delta\phi)$ and $\sin(2\Delta\phi)$ beam-spin asymmetries as a function of $P_{T1}P_{T2}$ with $0.2 \leq z_1 \leq 0.3$.

### F. Multidimensional $P_{T1}P_{T2}$-dependence of $\mathcal{A}_{LU}$ with $0.3 \leq z_1 \leq 0.4$

| Bin | $x$ Range | $< Q^2 >$ (GeV$^2$) | $< x >$ | $< y >$ | $< z_1 >$ | $< \zeta_2 >$ | $< P_{T1}P_{T2} >$ (GeV$^2$) | $< x_{F1} >$ | $< x_{F2} >$ | $< \Delta Y >$ |
|---|---|---|---|---|---|---|---|---|---|---|
| 1 | [0.1, 0.2] | 2.831 | 0.240 | 0.609 | 0.349 | 0.542 | 0.042 | 0.289 | -0.392 | 1.959 |
| 2 | (0.2, 0.3] | 2.731 | 0.229 | 0.618 | 0.347 | 0.541 | 0.100 | 0.266 | -0.349 | 1.563 |
| 3 | (0.3, 0.4] | 2.695 | 0.226 | 0.620 | 0.345 | 0.540 | 0.165 | 0.243 | -0.301 | 1.268 |
| 4 | (0.4, 0.5] | 2.657 | 0.220 | 0.626 | 0.345 | 0.544 | 0.231 | 0.224 | -0.270 | 1.080 |
| 5 | (0.5, 0.6] | 2.625 | 0.214 | 0.635 | 0.345 | 0.552 | 0.297 | 0.207 | -0.250 | 0.949 |
| 6 | (0.6, 0.7] | 2.577 | 0.206 | 0.644 | 0.345 | 0.562 | 0.363 | 0.192 | -0.237 | 0.851 |

TABLE XI: Average kinematic values for the bins of $P_{T1}P_{T2}$ with $0.3 \leq z_1 \leq 0.4$.

| Bin | $< P_{T1}P_{T2} >$ (GeV$^2$) | $\mathcal{A}_{LU}^{\sin(\Delta\phi)}$ | $\mathcal{A}_{LU}^{\sin(2\Delta\phi)}$ |
|---|---|---|---|
| 1 | 0.060 | $-0.011^{\pm 0.002}_{\pm 0.002}$ | $0.000^{\pm 0.002}_{\pm 0.001}$ |
| 2 | 0.147 | $-0.023^{\pm 0.003}_{\pm 0.003}$ | $0.001^{\pm 0.002}_{\pm 0.002}$ |
| 3 | 0.244 | $-0.037^{\pm 0.004}_{\pm 0.005}$ | $-0.004^{\pm 0.004}_{\pm 0.003}$ |
| 4 | 0.343 | $-0.061^{\pm 0.007}_{\pm 0.007}$ | $-0.017^{\pm 0.006}_{\pm 0.005}$ |
| 5 | 0.443 | $-0.047^{\pm 0.015}_{\pm 0.012}$ | $-0.011^{\pm 0.012}_{\pm 0.009}$ |
| 6 | 0.542 | $-0.010^{\pm 0.034}_{\pm 0.028}$ | $0.039^{\pm 0.025}_{\pm 0.020}$ |

TABLE XII: The mean value of $P_{T1}P_{T2}$ and the final beam-spin asymmetries as a function of $P_{T1}P_{T2}$ with $0.3 \leq z_1 \leq 0.4$ in each bin. Asymmetries are given as $\mathcal{A}_{LU}{}^{\Delta_{\rm stat}}_{\Delta_{\rm sys}}$.

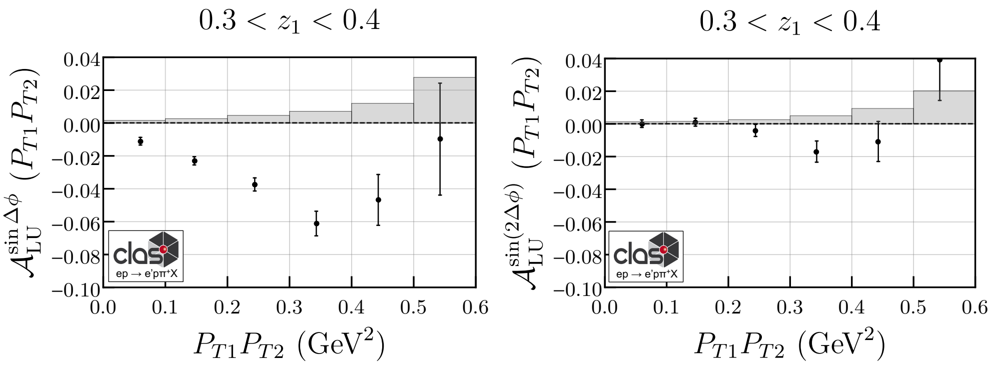


FIG. 6: The extracted amplitudes of the sin($\Delta\phi$) and sin($2\Delta\phi$) beam-spin asymmetries as a function of $P_{T1}P_{T2}$ with $0.3 \leq z_1 \leq 0.4$.

### G. Multidimensional $P_{T1}P_{T2}$-dependence of $\mathcal{A}_{LU}$ with $0.4 \leq z_1 \leq 0.5$

| Bin | $x$ Range | $< Q^2 >$ (GeV$^2$) | $< x >$ | $< y >$ | $< z_1 >$ | $< \zeta_2 >$ | $< P_{T1}P_{T2} >$ (GeV$^2$) | $< x_{F1} >$ | $< x_{F2} >$ | $< \Delta Y >$ |
|---|---|---|---|---|---|---|---|---|---|---|
| 1 | [0.1, 0.2] | 2.861 | 0.249 | 0.593 | 0.445 | 0.526 | 0.040 | 0.382 | -0.340 | 2.115 |
| 2 | (0.2, 0.3] | 2.749 | 0.232 | 0.612 | 0.443 | 0.531 | 0.099 | 0.365 | -0.315 | 1.753 |
| 3 | (0.3, 0.4] | 2.650 | 0.219 | 0.626 | 0.443 | 0.537 | 0.164 | 0.348 | -0.295 | 1.508 |
| 4 | (0.4, 0.5] | 2.583 | 0.210 | 0.636 | 0.443 | 0.542 | 0.231 | 0.332 | -0.277 | 1.332 |
| 5 | (0.5, 0.6] | 2.539 | 0.203 | 0.644 | 0.443 | 0.550 | 0.297 | 0.317 | -0.263 | 1.201 |
| 6 | (0.6, 0.7] | 2.495 | 0.198 | 0.650 | 0.443 | 0.558 | 0.364 | 0.303 | -0.251 | 1.096 |

TABLE XIII: Average kinematic values for the bins of $P_{T1}P_{T2}$ with $0.4 \leq z_1 \leq 0.5$.

| Bin | $< P_{T1}P_{T2} >$ (GeV$^2$) | $\mathcal{A}_{LU}^{\sin(\Delta\phi)}$ | $\mathcal{A}_{LU}^{\sin(2\Delta\phi)}$ |
|---|---|---|---|
| 1 | 0.057 | $-0.010^{\pm 0.003}_{\pm 0.002}$ | $-0.002^{\pm 0.003}_{\pm 0.002}$ |
| 2 | 0.145 | $-0.016^{\pm 0.003}_{\pm 0.002}$ | $-0.002^{\pm 0.003}_{\pm 0.002}$ |
| 3 | 0.244 | $-0.029^{\pm 0.006}_{\pm 0.005}$ | $-0.002^{\pm 0.005}_{\pm 0.004}$ |
| 4 | 0.344 | $-0.054^{\pm 0.012}_{\pm 0.009}$ | $-0.017^{\pm 0.010}_{\pm 0.007}$ |
| 5 | 0.444 | $-0.055^{\pm 0.027}_{\pm 0.020}$ | $0.002^{\pm 0.020}_{\pm 0.015}$ |
| 6 | 0.544 | $-0.094^{\pm 0.168}_{\pm 0.055}$ | $-0.030^{\pm 0.203}_{\pm 0.037}$ |

TABLE XIV: The mean value of $P_{T1}P_{T2}$ and the final beam-spin asymmetries as a function of $P_{T1}P_{T2}$ with $0.4 \leq z_1 \leq 0.5$ in each bin. Asymmetries are given as $\mathcal{A}_{LU}{}^{\Delta_{\rm stat}}_{\Delta_{\rm sys}}$.

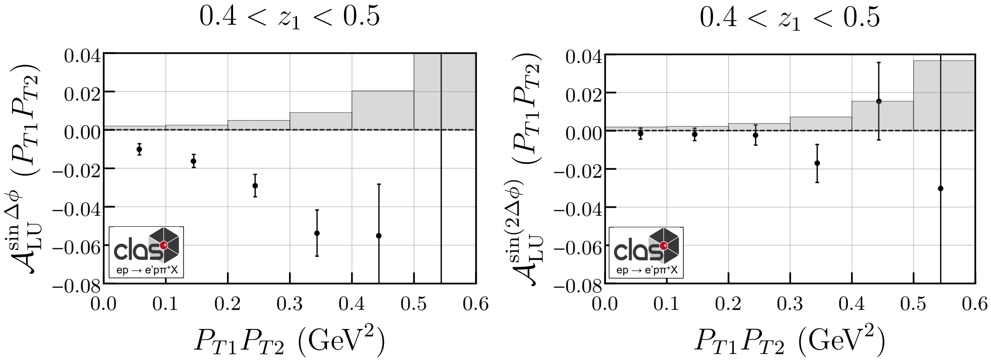


FIG. 7: The extracted amplitudes of the sin($\Delta\phi$) and sin($2\Delta\phi$) beam-spin asymmetries as a function of $P_{T1}P_{T2}$ with $0.4 \leq z_1 \leq 0.5$.

### H. Multidimensional $P_{T1}P_{T2}$-dependence of $\mathcal{A}_{LU}$ with $0.5 \leq z_1 \leq 0.6$

| Bin | $x$ Range | $< Q^2 >$ (GeV$^2$) | $< x >$ | $< y >$ | $< z_1 >$ | $< \zeta_2 >$ | $< P_{T1}P_{T2} >$ (GeV$^2$) | $< x_{F1} >$ | $< x_{F2} >$ | $< \Delta Y >$ |
|---|---|---|---|---|---|---|---|---|---|---|
| 1 | [0.1, 0.2] | 2.711 | 0.236 | 0.592 | 0.537 | 0.524 | 0.039 | 0.472 | -0.320 | 2.309 |
| 2 | (0.2, 0.3] | 2.579 | 0.217 | 0.613 | 0.535 | 0.532 | 0.098 | 0.458 | -0.310 | 1.948 |
| 3 | (0.3, 0.4] | 2.482 | 0.204 | 0.627 | 0.534 | 0.538 | 0.164 | 0.443 | -0.298 | 1.698 |
| 4 | (0.4, 0.5] | 2.419 | 0.196 | 0.635 | 0.533 | 0.545 | 0.231 | 0.427 | -0.286 | 1.522 |
| 5 | (0.5, 0.6] | 2.371 | 0.190 | 0.642 | 0.532 | 0.552 | 0.297 | 0.414 | -0.271 | 1.386 |
| 6 | (0.6, 0.7] | 2.331 | 0.184 | 0.650 | 0.531 | 0.560 | 0.364 | 0.401 | -0.262 | 1.283 |

TABLE XV: Average kinematic values for the bins of $P_{T1}P_{T2}$ with $0.5 \leq z_1 \leq 0.6$.

| Bin | $< P_{T1}P_{T2} >$ (GeV$^2$) | $\mathcal{A}_{LU}^{\sin(\Delta\phi)}$ | $\mathcal{A}_{LU}^{\sin(2\Delta\phi)}$ |
|---|---|---|---|
| 1 | 0.055 | $-0.002^{\pm0.005}_{\pm0.003}$ | $0.002^{\pm0.005}_{\pm0.003}$ |
| 2 | 0.144 | $-0.003^{\pm0.006}_{\pm0.005}$ | $0.011^{\pm0.006}_{\pm0.005}$ |
| 3 | 0.244 | $-0.016^{\pm0.014}_{\pm0.010}$ | $-0.002^{\pm0.011}_{\pm0.009}$ |
| 4 | 0.344 | $-0.004^{\pm0.028}_{\pm0.026}$ | $0.009^{\pm0.021}_{\pm0.019}$ |
| 5 | 0.443 | $-0.088^{\pm0.178}_{\pm0.076}$ | $-0.002^{\pm0.249}_{\pm0.049}$ |
| 6 | 0.543 | $0.051^{\pm0.062}_{\pm0.212}$ | $0.040^{\pm0.042}_{\pm0.123}$ |

TABLE XVI: The mean value of $P_{T1}P_{T2}$ and the final beam-spin asymmetries as a function of $P_{T1}P_{T2}$ with $0.5 \leq z_1 \leq 0.6$ in each bin. Asymmetries are given as $\mathcal{A}_{LU}{}^{\Delta_{\rm stat}}_{\Delta_{\rm sys}}$.

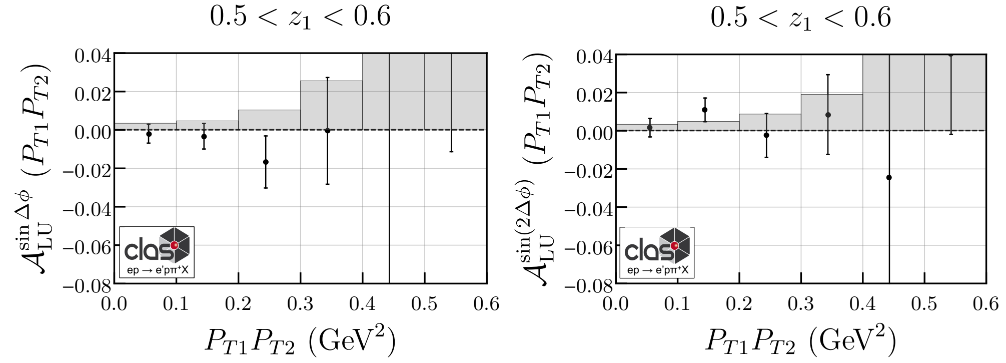


FIG. 8: The extracted amplitudes of the $\sin(\Delta\phi)$ and $\sin(2\Delta\phi)$ beam-spin asymmetries as a function of $P_{T1}P_{T2}$ with $0.5 \leq z_1 \leq 0.6$.

## I. $x_{F2}$-dependence of $\mathcal{A}_{LU}$

| Bin | $x$ Range | $< Q^2 >$ (GeV$^2$) | $< x >$ | $< y >$ | $< z_1 >$ | $< \zeta_2 >$ | $< P_{T1}P_{T2} >$ (GeV$^2$) | $< x_{F1} >$ | $< x_{F2} >$ | $< \Delta Y >$ |
|---|---|---|---|---|---|---|---|---|---|---|
| 1 | [-0.82, -0.60] | 2.805 | 0.219 | 0.657 | 0.310 | 0.654 | 0.083 | 0.244 | -0.638 | 2.007 |
| 2 | (-0.60, -0.38] | 2.674 | 0.217 | 0.637 | 0.332 | 0.588 | 0.138 | 0.243 | -0.468 | 1.633 |
| 3 | (-0.38, -0.16] | 2.639 | 0.217 | 0.631 | 0.347 | 0.532 | 0.194 | 0.238 | -0.277 | 1.253 |
| 4 | (-0.16, 0.06] | 2.652 | 0.220 | 0.626 | 0.343 | 0.505 | 0.252 | 0.205 | -0.071 | 0.763 |
| 5 | (0.06, 0.28] | 2.679 | 0.221 | 0.627 | 0.301 | 0.516 | 0.295 | 0.125 | 0.138 | 0.166 |
| 6 | (0.28, 0.50] | 2.604 | 0.208 | 0.645 | 0.253 | 0.561 | 0.291 | 0.056 | 0.345 | -0.328 |

TABLE XVII: Average kinematic values for the bins of $x_{F2}$.

| Bin | $< x_{F2} >$ | $\mathcal{A}_{LU}^{\sin(\Delta\phi)}$ | $\mathcal{A}_{LU}^{\sin(2\Delta\phi)}$ |
|---|---|---|---|
| 1 | -0.638 | $0.010^{\pm 0.005}_{\pm 0.004}$ | $-0.005^{\pm 0.005}_{\pm 0.003}$ |
| 2 | -0.467 | $-0.012^{\pm 0.001}_{\pm 0.001}$ | $0.001^{\pm 0.001}_{\pm 0.001}$ |
| 3 | -0.277 | $-0.022^{\pm 0.001}_{\pm 0.001}$ | $0.000^{\pm 0.001}_{\pm 0.001}$ |
| 4 | -0.071 | $-0.030^{\pm 0.003}_{\pm 0.001}$ | $-0.001^{\pm 0.002}_{\pm 0.001}$ |
| 5 | 0.138 | $-0.053^{\pm 0.009}_{\pm 0.002}$ | $-0.009^{\pm 0.007}_{\pm 0.001}$ |
| 6 | 0.345 | $-0.077^{\pm 0.031}_{\pm 0.004}$ | $-0.013^{\pm 0.023}_{\pm 0.003}$ |

TABLE XVIII: The mean value of $x_{F2}$ and the final beam-spin asymmetries as a function of $x_{F2}$ in each bin. Asymmetries are given as $\mathcal{A}_{LU}{}^{\Delta_{\rm stat}}_{\Delta_{\rm sys}}$.

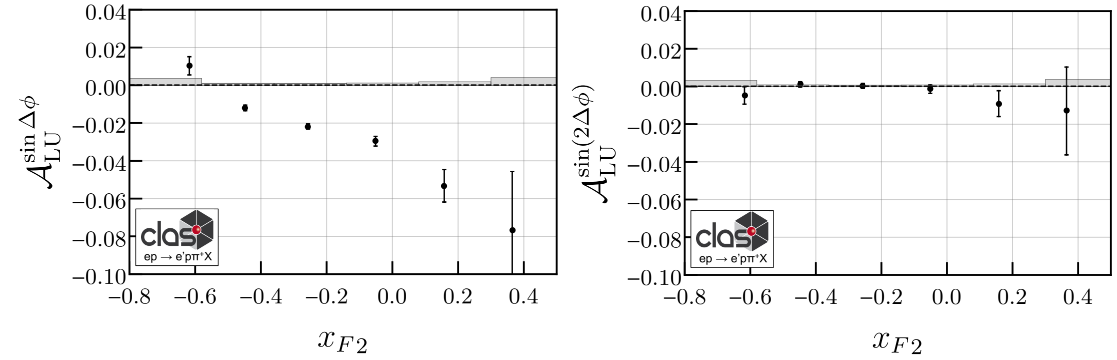


FIG. 9: The extracted amplitudes of the sin($\Delta\phi$) and sin($2\Delta\phi$) beam-spin asymmetries as a function of $x_{F2}$.

### J. $\Delta Y$-dependence of $\mathcal{A}_{LU}$

| Bin | $x$ Range | $< Q^2 >$ (GeV$^2$) | $< x >$ | $< y >$ | $< z_1 >$ | $< \zeta_2 >$ | $< P_{T1}P_{T2} >$ (GeV$^2$) | $< x_{F1} >$ | $< x_{F2} >$ | $< \Delta Y >$ |
|---|---|---|---|---|---|---|---|---|---|---|
| 1 | [-1.00, -0.33] | 2.763 | 0.222 | 0.639 | 0.234 | 0.527 | 0.310 | -0.044 | 0.268 | -0.487 |
| 2 | (-0.33, 0.33] | 2.775 | 0.230 | 0.624 | 0.267 | 0.511 | 0.329 | 0.051 | 0.027 | 0.097 |
| 3 | (0.33, 1.00] | 2.667 | 0.220 | 0.629 | 0.306 | 0.529 | 0.272 | 0.155 | -0.192 | 0.714 |
| 4 | (1.00, 1.67] | 2.619 | 0.214 | 0.636 | 0.344 | 0.553 | 0.174 | 0.249 | -0.335 | 1.321 |
| 5 | (1.67, 2.33] | 2.669 | 0.218 | 0.633 | 0.378 | 0.565 | 0.091 | 0.321 | -0.398 | 1.947 |
| 6 | (2.33, 3.00] | 2.671 | 0.216 | 0.637 | 0.432 | 0.579 | 0.043 | 0.386 | -0.453 | 2.537 |

TABLE XIX: Average kinematic values for the bins of $\Delta Y$.

| Bin | $< \Delta Y >$ | $\mathcal{A}_{LU}^{\sin(\Delta\phi)}$ | $\mathcal{A}_{LU}^{\sin(2\Delta\phi)}$ |
|---|---|---|---|
| 1 | -0.487 | $-0.035^{\pm 0.012}_{\pm 0.018}$ | $0.014^{\pm 0.014}_{\pm 0.007}$ |
| 2 | 0.097 | $-0.032^{\pm 0.002}_{\pm 0.006}$ | $-0.003^{\pm 0.005}_{\pm 0.001}$ |
| 3 | 0.714 | $-0.024^{\pm 0.001}_{\pm 0.003}$ | $0.001^{\pm 0.002}_{\pm 0.001}$ |
| 4 | 1.321 | $-0.025^{\pm 0.001}_{\pm 0.001}$ | $0.000^{\pm 0.001}_{\pm 0.001}$ |
| 5 | 1.947 | $-0.010^{\pm 0.001}_{\pm 0.002}$ | $0.000^{\pm 0.002}_{\pm 0.001}$ |
| 6 | 2.537 | $-0.003^{\pm 0.004}_{\pm 0.004}$ | $-0.005^{\pm 0.003}_{\pm 0.002}$ |

TABLE XX: The mean value of $\Delta Y$ and the final beam-spin asymmetries as a function of $\Delta Y$ in each bin. Asymmetries are given as $\mathcal{A}_{LU}{}^{\Delta_{\rm stat}}_{\Delta_{\rm sys}}$.

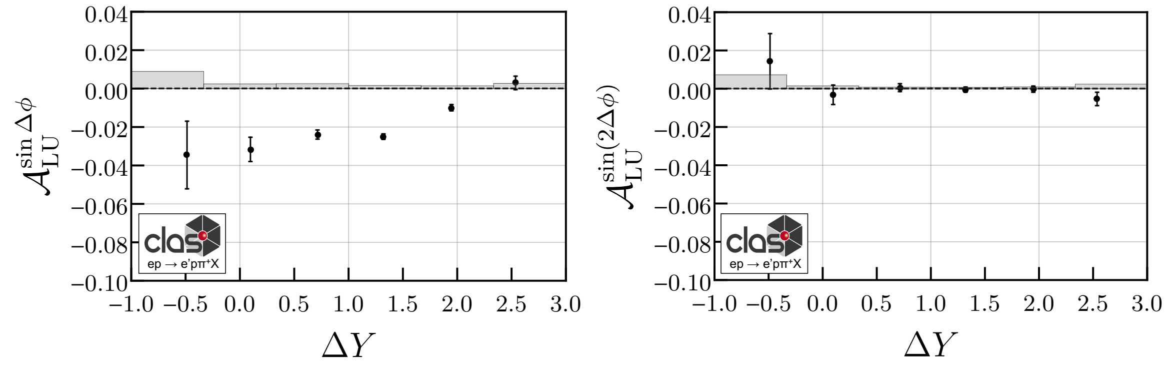


FIG. 10: The extracted amplitudes of the sin($\Delta\phi$) and sin($2\Delta\phi$) beam-spin asymmetries as a function of $\Delta Y$.

### K. $M_x(ep \to e'p\pi^+X)$-dependence of $\mathcal{A}_{LU}$

| Bin | $x$ Range | $< Q^2 >$ (GeV$^2$) | $< x >$ | $< y >$ | $< z_1 >$ | $< \zeta_2 >$ | $< P_{T1}P_{T2} >$ (GeV$^2$) | $< x_{F1} >$ | $< x_{F2} >$ | $< \Delta Y >$ |
|---|---|---|---|---|---|---|---|---|---|---|
| 1 | [0.00, 0.25] | 3.539 | 0.389 | 0.468 | 0.540 | 0.577 | 0.235 | 0.375 | -0.414 | 1.401 |
| 2 | (0.25, 0.50] | 3.503 | 0.372 | 0.485 | 0.503 | 0.573 | 0.210 | 0.353 | -0.417 | 1.434 |
| 3 | (0.50, 0.75] | 3.305 | 0.330 | 0.516 | 0.466 | 0.568 | 0.201 | 0.329 | -0.384 | 1.419 |
| 4 | (0.75, 1.00] | 3.125 | 0.287 | 0.558 | 0.415 | 0.567 | 0.196 | 0.292 | -0.370 | 1.402 |
| 5 | (1.00, 1.25] | 2.876 | 0.244 | 0.603 | 0.370 | 0.560 | 0.190 | 0.259 | -0.343 | 1.369 |
| 6 | (1.25, 1.50] | 2.600 | 0.207 | 0.644 | 0.332 | 0.550 | 0.179 | 0.233 | -0.316 | 1.343 |
| 7 | (1.50, 1.75] | 2.310 | 0.174 | 0.680 | 0.298 | 0.535 | 0.163 | 0.209 | -0.281 | 1.299 |
| 8 | (1.75, 2.00] | 2.023 | 0.146 | 0.709 | 0.269 | 0.515 | 0.142 | 0.191 | -0.240 | 1.251 |
| 9 | (2.00, 2.25] | 1.740 | 0.121 | 0.730 | 0.246 | 0.494 | 0.119 | 0.178 | -0.197 | 1.206 |
| 10 | (2.25, 2.50] | 1.349 | 0.091 | 0.746 | 0.229 | 0.482 | 0.080 | 0.180 | -0.195 | 1.366 |

TABLE XXI: Average kinematic values for the bins of $M_x$.

| Bin | $< M_x >$ (GeV) | $\mathcal{A}_{LU}^{\sin(\Delta\phi)}$ | $\mathcal{A}_{LU}^{\sin(2\Delta\phi)}$ |
|---|---|---|---|
| 1 | 0.163 | $-0.023^{\pm 0.003}_{\pm 0.015}$ | $0.013^{\pm 0.003}_{\pm 0.004}$ |
| 2 | 0.385 | $-0.007^{\pm 0.003}_{\pm 0.005}$ | $-0.001^{\pm 0.002}_{\pm 0.003}$ |
| 3 | 0.639 | $-0.004^{\pm 0.002}_{\pm 0.002}$ | $0.000^{\pm 0.002}_{\pm 0.001}$ |
| 4 | 0.875 | $-0.016^{\pm -0.002}_{\pm 0.001}$ | $-0.001^{\pm 0.002}_{\pm 0.001}$ |
| 5 | 1.127 | $-0.019^{\pm 0.002}_{\pm 0.001}$ | $-0.002^{\pm 0.001}_{\pm 0.001}$ |
| 6 | 1.368 | $-0.019^{\pm 0.002}_{\pm 0.001}$ | $0.000^{\pm 0.002}_{\pm 0.001}$ |
| 7 | 1.609 | $-0.014^{\pm 0.002}_{\pm 0.001}$ | $0.000^{\pm 0.002}_{\pm 0.001}$ |
| 8 | 1.846 | $-0.012^{\pm 0.004}_{\pm 0.002}$ | $0.008^{\pm 0.004}_{\pm 0.002}$ |
| 9 | 2.053 | $-0.009^{\pm 0.019}_{\pm 0.005}$ | $0.002^{\pm 0.017}_{\pm 0.005}$ |
| 10 | 2.263 | $-0.019^{\pm 0.234}_{\pm 0.041}$ | $0.134^{\pm 0.303}_{\pm 0.042}$ |

TABLE XXII: The mean value of $M_x$ and the final beam-spin asymmetries as a function of $M_x$ in each bin. Asymmetries are given as $\mathcal{A}_{LU}{}^{\Delta_{\text{stat}}}_{\Delta_{\text{sys}}}$.

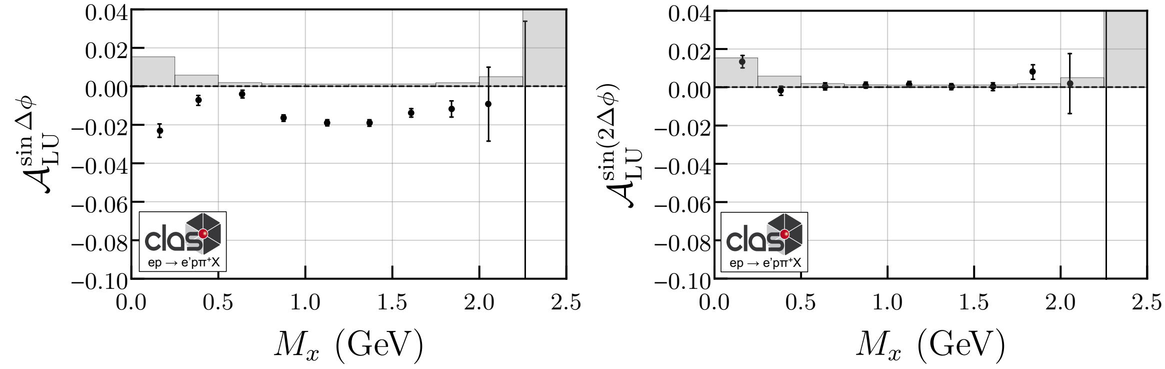


FIG. 11: The extracted amplitudes of the $\sin(\Delta\phi)$ and $\sin(2\Delta\phi)$ beam-spin asymmetries as a function of $M_x$.

### L. Monte Carlo

The experimental configuration has been described in detail in GEMC [2], a GEANT4 based simulation package that offers the possibility to easily implement detectors in a full GEANT simulation. The position of the CLAS12 detectors in Hall B at JLab have been matched to survey data and a realistic map of the magnetic field has been generated to accurately reproduce the experimental set up. LUND generators were used to produce realistic final states that were read by GEMC version 4.3.2 and passed through the detector system of CLAS12.

The generator used for this analysis is called clasdis [3], which is based on the PEPSI generator [4, 5], the polarized version of the well-known LEPTO generator [6]. The generator is specific to SIDIS processes and so is missing other interactions such as photo-production. The parton-level interaction is based on electroweak cross sections. First-order QCD matrix elements for boson-gluon fusion and gluon radiation are implemented. The hadronization process follows the LUND string model implemented in Pythia (Jetset). Parameters changed to reproduce the electron, photon and pion distributions obtained from data are: PARJ(21), defining the average intrinsic transverse momentum (from default 0.36 to 0.5 GeV), PARJ(11), defining the fraction of spin 1 light mesons (from default 0.5 to 0.7) and PARJ(12) defining the fraction of spin 1 strange mesons (from default 0.6 to 0.75). Those changes are consistent with the latest measurements of dihadron distributions at CLAS12.

The integrated-over-all-other variables $Q^2$, $x$, $x_{F2}$ and $P_{T1}P_{T2}$ distributions are shown in Fig. 12

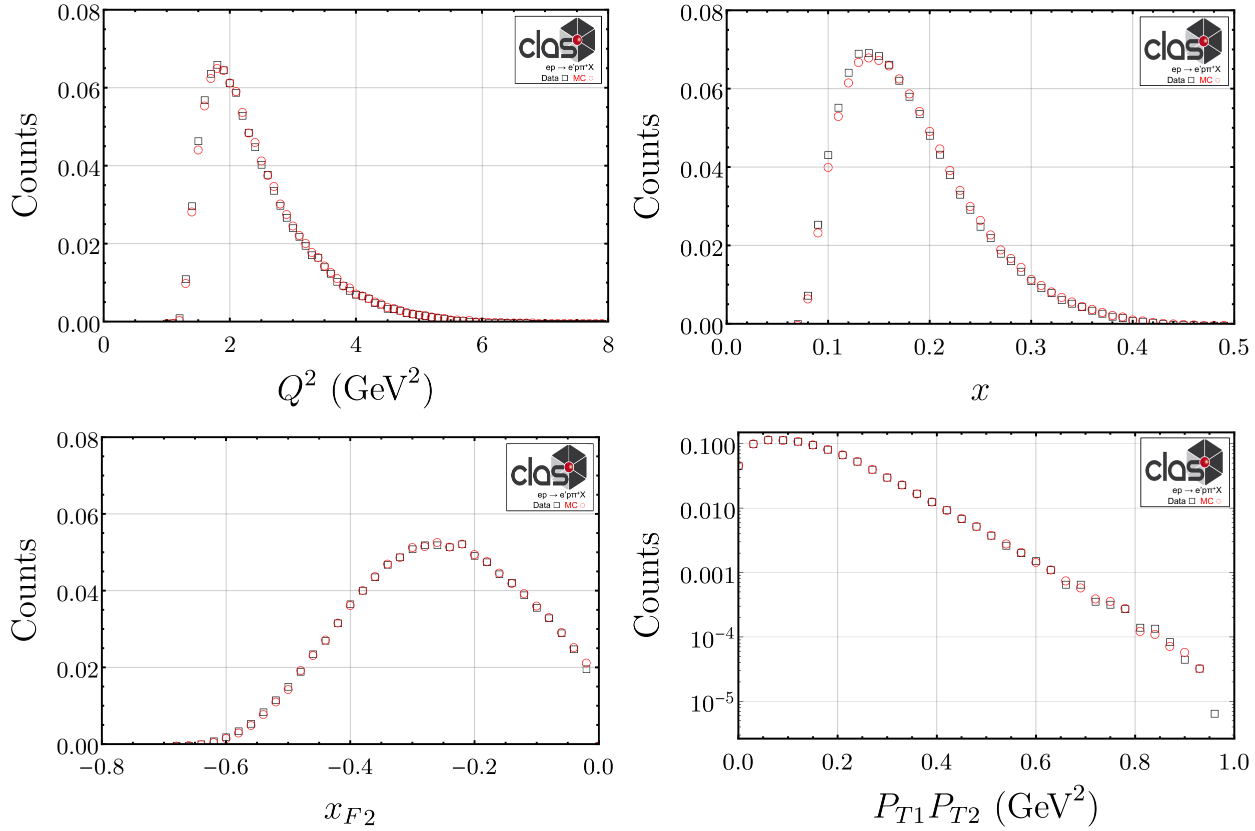


FIG. 12: Comparison between data (black squares) and Monte Carlo (red circles) for $Q^2$ (top left), $x$ (top right), $x_{F2}$ (bottom left) and $P_{T1}P_{T2}$ (bottom right, log scale). Counts are normalized to the total number of dihadron pairs. Excellent agreement is observed.

for the data (black) and Monte Carlo (red). Almost exact agreement is observed.

[1] M. Anselmino, V. Barone, and A. Kotzinian, Phys. Lett. B **713**, 317 (2012), arXiv:1112.2604 [hep-ph].

[2] M. Ungaro *et al.*, Nucl. Instrum. Meth. A **959**, 163422 (2020).

[3] H. Avakian, "clasdis," `https://github.com/JeffersonLab/clasdis` (2020).

[4] T. Sjostrand, S. Mrenna, and P. Z. Skands, JHEP **0605**, 026 (2006), arXiv:hep-ph/0603175 [hep-ph].

[5] L. Mankiewicz, A. Schafer, and M. Veltri, Comput. Phys. Commun. **71**, 305 (1992).

[6] G. Ingelman, A. Edin, and J. Rathsman, Comput.Phys.Commun. **101**, 108 (1997), arXiv:hep-ph/9605286 [hep-ph].
